# Supplementary material for: Cross-View Image Synthesis using Conditional GANs
Source: arXiv:1803.03396 source file (2018-03-29)
Supplement: Supplementary file 1 [file supplementary-materials-cross.pdf]

# Supplementary Materials: Cross-View Image Synthesis using Conditional GANs

Krishna Regmi and Ali Borji
Center for Research in Computer Vision (CRCV), University of Central Florida (UCF)
kregmi@knights.ucf.edu, aborji@crcv.ucf.edu

This supplementary material elaborates the network architectures and provides in-depth analysis of the qualitative cross-view generation results on two challenging datasets.

## 1. Network Structures

In Table 1, we present details of encoder and decoder used for higher resolution (256×256) image generation. This includes the operations involved in each layer as well the size of output after each block.

For the baseline method (Pix2pix [2]), the generator is an encoder-decoder network. The generator of X-Fork method has a single encoder and two symmetrical decoders; one for image synthesis and the other for segmentation map synthesis. The decoders share weights except for the final two layers. For X-Seq architecture, we have a sequence of two GANs; the generators are encoder-decoder networks same as the baseline.

The discriminators used in all three methods have common architecture. It is similar to the encoder part of generator except that dropout layers are not used and the final activation layer is Sigmoid instead of Tanh.

For lower resolution (64×64) experiments, $CBL_7$ and $CBL_8$ blocks are removed from encoder, and $UBDR_1$ and $UBDR_2$ are dropped from decoder. Since the input resolution is reduced by 4, the second and third values of 'output size' in the table also get reduced by four.

Table 1: Network Details of encoder and decoder used in GANs. Different operations carried out at each block are shown along with output dimensions.

| G | Block | Operations | Output Size |
|---|---|---|---|
| | $CL_1$ | Conv, lReLU | 64×128×128 |
| **e** | $CBL_2$ | Conv, BN, lReLU | 128×64×64 |
| **n** | $CBL_3$ | Conv, BN, lReLU | 256×32×32 |
| **c** | $CBL_4$ | Conv, BN, lReLU | 512×16×16 |
| **o** | $CBL_5$ | Conv, BN, lReLU | 512×8×8 |
| **d** | $CBL_6$ | Conv, BN, lReLU | 512×4×4 |
| **e** | $CBL_7$ | Conv, BN, lReLU | 512×2×2 |
| **r** | $CBL_8$ | Conv, BN, lReLU | 512×1×1 |
| | $UBDR_1$ | UpConv, BN, Dropout, ReLU | 512×2×2 |
| **d** | $UBDR_2$ | UpConv, BN, Dropout, ReLU | 512×4×4 |
| **e** | $UBDR_3$ | UpConv, BN, Dropout, ReLU | 512×8×8 |
| **c** | $UBR_4$ | UpConv, BN, ReLU | 512×16×16 |
| **o** | $UBR_5$ | UpConv, BN, ReLU | 256×32×32 |
| **d** | $UBR_6$ | UpConv, BN, ReLU | 128×64×64 |
| **e** | $UBR_7$ | UpConv, BN, ReLU | 64×128×128 |
| **r** | $UT_8$ | UpConv, Tanh | 3×256×256 |

## 2. Effectiveness of Semantic Segmentation

Figure 1 shows the effectiveness of our methods in generating semantic segmentation in target view conditioned on images from the source view. The segmentation maps obtained by using state-of-the-art RefineNet [3] pretrained on Cityscapes dataset [1] overlaid on real image pairs are shown in second column. These semantic maps have pixel labels from 20 classes ('road', 'sidewalk', 'building', 'wall', 'fence', 'pole', 'trafficlight', 'trafficsign', 'vegetation', 'terrain', 'sky', 'person', 'rider', 'car', 'truck', 'bus', 'train', 'motorcycle', 'bicycle', 'void'). Most common classes in Dayton dataset are: road, sidewalk, building, vegetation, terrain, sky, etc. The segmentation maps for aerial images show missed classification ('void' class) for road, buildings, cars in images of row 2, 3 and 6. This is because RefineNet was primarily trained on street-view images and is tested on aerial images here. Similarly, the segmentation maps generated by proposed methods are overlaid on image pairs and illustrated in third and fourth columns respectively.

On ground level segmentations, our methods perform well to capture sky, road, terrain and vegetation. This is best represented in rows 1 and 4. Images in row 6 show trees misclassified as sky at top right corner by X-Seq method and is better classified by X-Fork. The aerial image segmentation has some misclassification. The images in row 1 show road is classified as void by X-Fork, as in its ground truth segmentation from RefineNet, whereas it is classified as vegetation by X-Seq. Images in row 3, 4 and 6 show road and buildings are missed in ground truth segmentation. The roads are partially segmented for images of row 3 and the methods do pretty good for row 4. The problem still exists in generated segmentations of row 6.

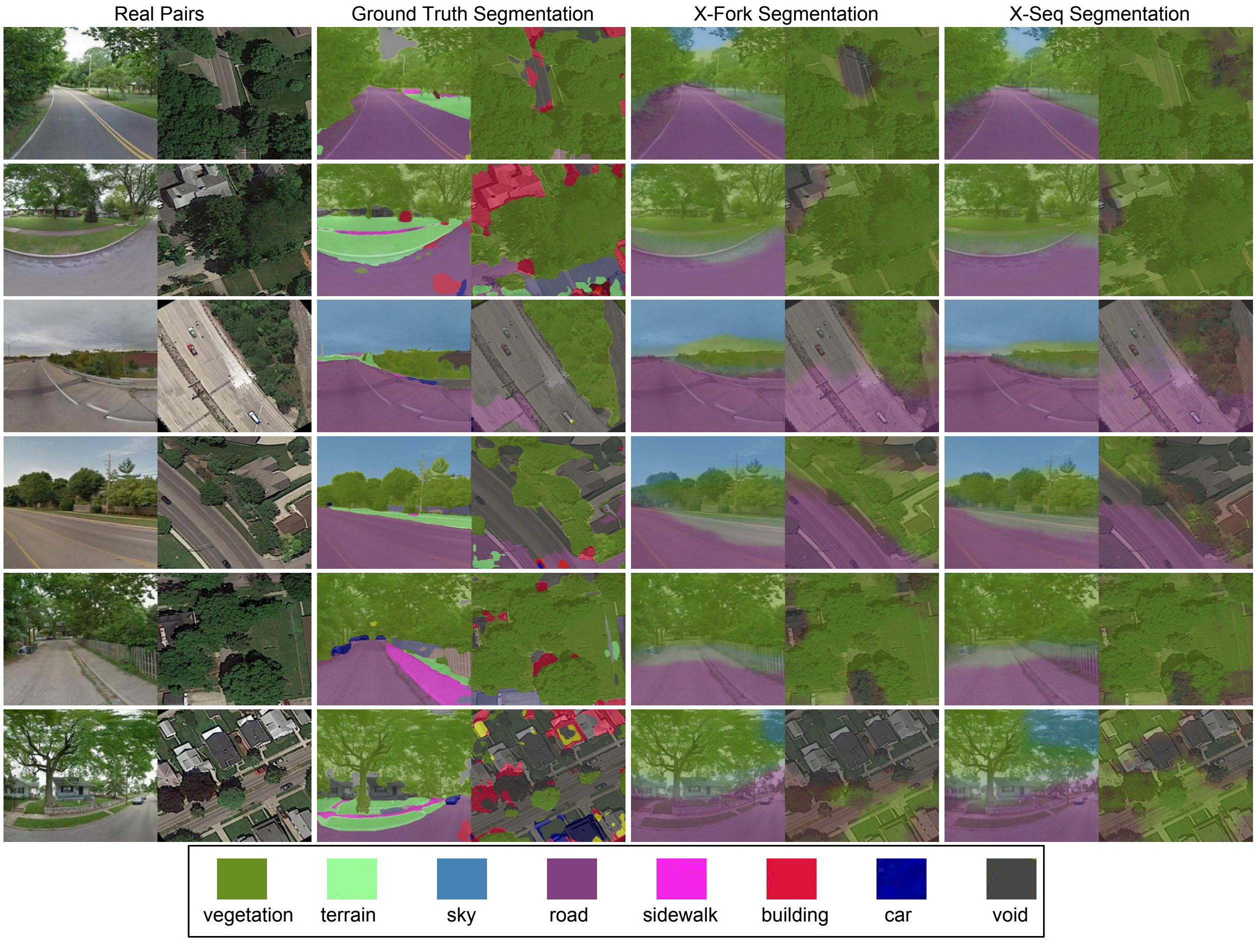


Figure 1: Segmentation overlay: Original image pairs are shown in first column, second column shows segmentation maps obtained from RefineNet [3] overlaid on original images. The next two columns have segmentation maps from our proposed X-Fork and X-Seq methods overlaid on original images. The color representation of common semantic classes from Dayton dataset are provided below the images.

The generation of aerial segmentation is more challenging because all object classes may not be visible in street-view images. This normally happens when we have many objects in aerial view images that are occluded in street-view. It is the same reason why our methods work well in images of row 4 but not for images of row 6.

## 3. Qualitative Evaluation

For qualitative analysis, we illustrate the images generated by different methods in **a2g** and **g2a** directions on both datasets. The qualitative results show the superiority of our generative architectures over existing methods.

Figure 2 displays the qualitative results on Dayton dataset for aerial to ground (**a2g**) synthesis. We observe that addition of $L1$ loss between real and generated semantic segmentation images while training our networks helps to generate images that are semantically related to ground truth compared to Pix2pix[2]. Images in rows 1, 3, 4, 5, 6 and 8 show that the proposed methods are successful at generating roads at correct locations. Houses are generated with structural details in images of rows 1, 5, 7 and 8. Sidewalks are well represented in generated images of rows 7 and 8. X-Fork learns to synthesize cars in images of rows 1 and 3. X-Seq tries to generate car in rows 1, 7 and 8.

The ground to aerial (**g2a**) generation on Dayton dataset is shown in Figure 4. The street-view image has house on right side of road and the X-Seq method is able to generate the house even though it is not present in ground truth image. But the numerous cars present in the true aerial image do not have correspondence in street-view image. So, they are not generated by the methods. The networks have learned to generate shadows as seen around trees in second row images. The ground truth aerial image in second row does not show the house that is visible in conditioning street-view image. So, the houses are present in images generated by all three methods. Images in rows 2, 5 and 7

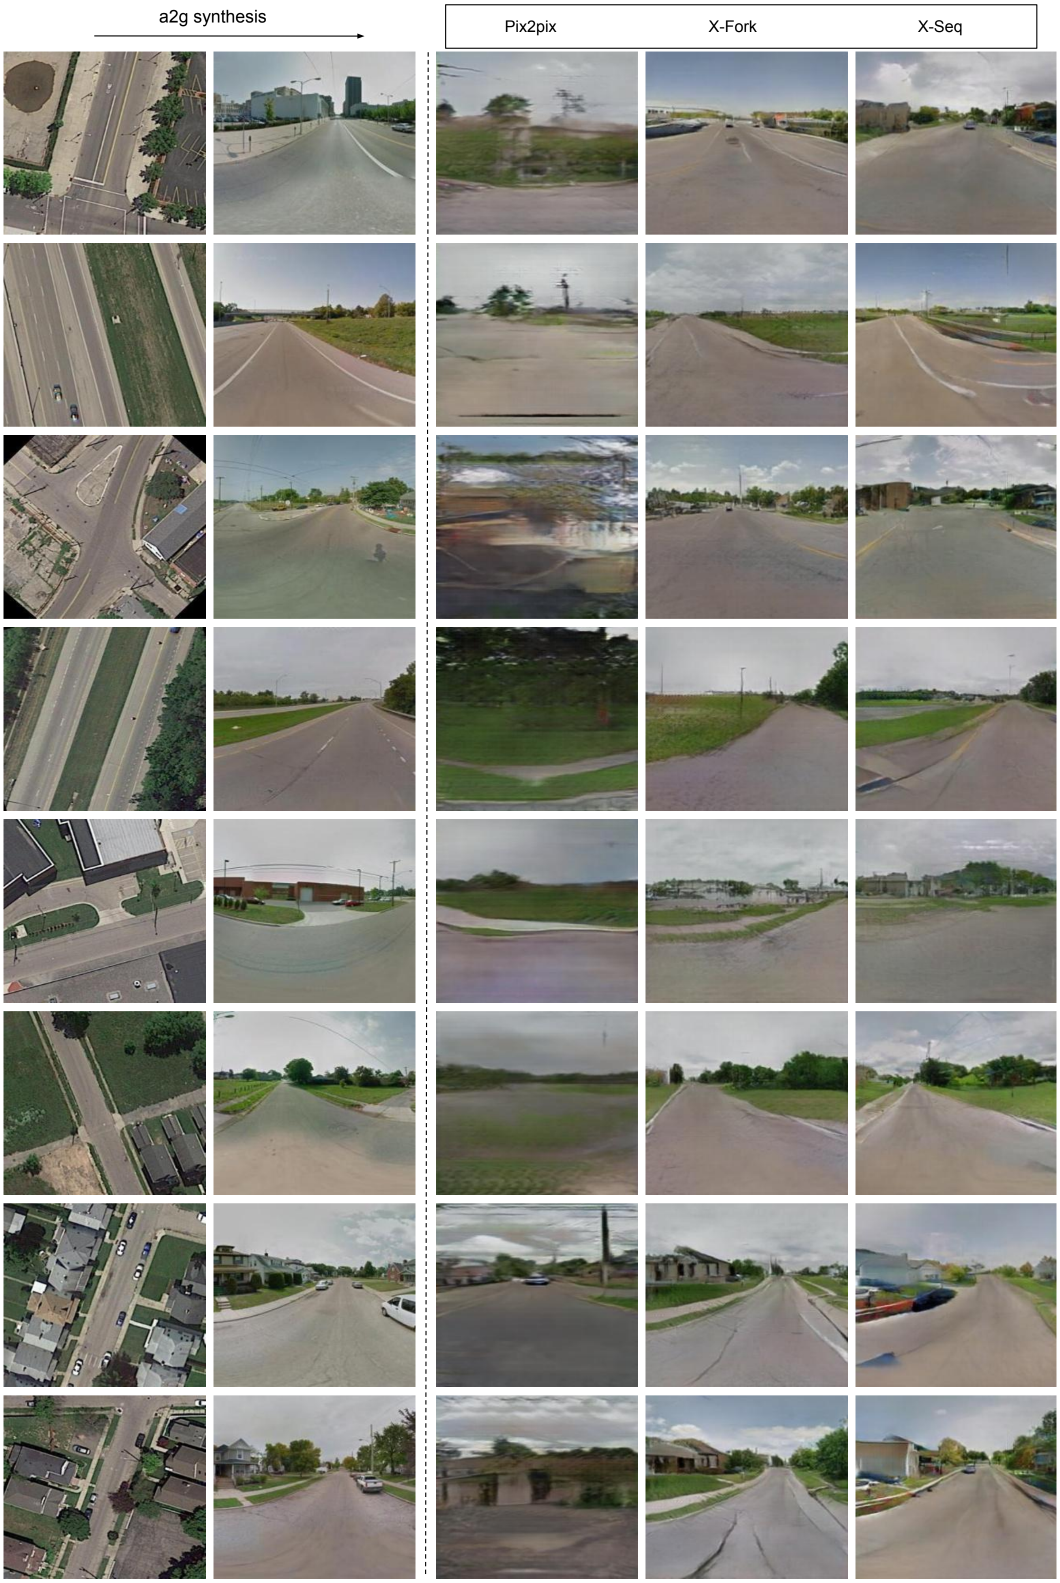


Figure 2: Qualitative results for Aerial to Ground level (**a2g**) synthesis using different methods on Dayton dataset. The networks learn to generate road, sidewalk (rows 2, 5, 7, 8), trees, houses (rows 1, 3, 5, 7, 8), pole (rows 2, 3, 4, 5) in the images.

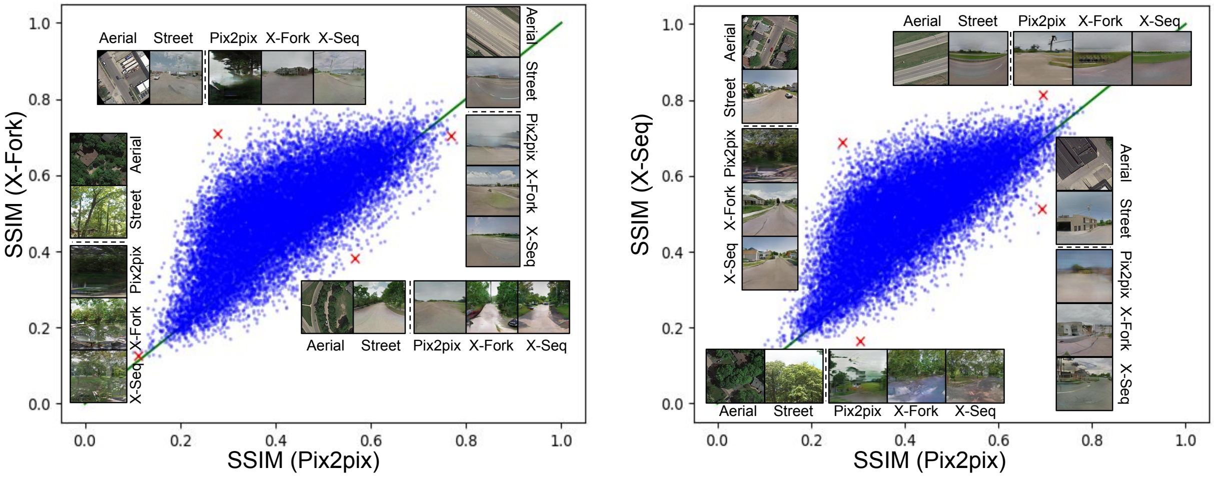


(a) Scatterplot: X-Fork vs Pix2pix

(b) Scatterplot: X-Seq vs Pix2pix

Figure 3: Scatterplot of SSIM scores obtained using different methods for test images of Dayton dataset. Images are shown at different points of scatterplot.

show the X-Fork network has learned to generate cars.

The generated images in aerial view look more distorted primarily because the generated roads are not parallel at edges. This is due to occlusions of road by trees in the aerial images. The major challenge in **g2a** synthesis is that networks need to estimate the scene beyond the small field of view of ground level image. The generated images should preserve the homogeneity of structures in the scene. This causes greater discrepancy between real and generated images in outer regions of images.

The qualitative results for **a2g** generation on CVUSA dataset are visualized in Figure 5. Our proposed methods generate much better images than Zhai et al. [4] and Pix2pix [2]. The proposed networks are successful at capturing the semantic information in aerial images and transforming them to the target view.

For further evaluation, we generate the scatter plots of SSIM scores of 21048 test images of Dayton dataset in Figure 3. The scatter plots show the superiority of our proposed method over the baseline. The images at few **x** points are shown in scatterplots. The generated images look similar to the ground truth even for points where SSIM values are low.

## References

[1] M. Cordts, M. Omran, S. Ramos, T. Rehfeld, M. Enzweiler, R. Benenson, U. Franke, S. Roth, and B. Schiele. The cityscapes dataset for semantic urban scene understanding. In *Proc. of the IEEE Conference on Computer Vision and Pattern Recognition (CVPR)*, 2016. 1

[2] P. Isola, J.-Y. Zhu, T. Zhou, and A. A. Efros. Image-to-image translation with conditional adversarial networks. *CVPR*, 2017. 1, 2, 4

[3] G. Lin, A. Milan, C. Shen, and I. Reid. RefineNet: Multi-path refinement networks for high-resolution semantic segmentation. In *CVPR*, July 2017. 1, 2

[4] M. Zhai, Z. Bessinger, S. Workman, and N. Jacobs. Predicting ground-level scene layout from aerial imagery. In *IEEE Conference on Computer Vision and Pattern Recognition (CVPR)*, 2017. 4

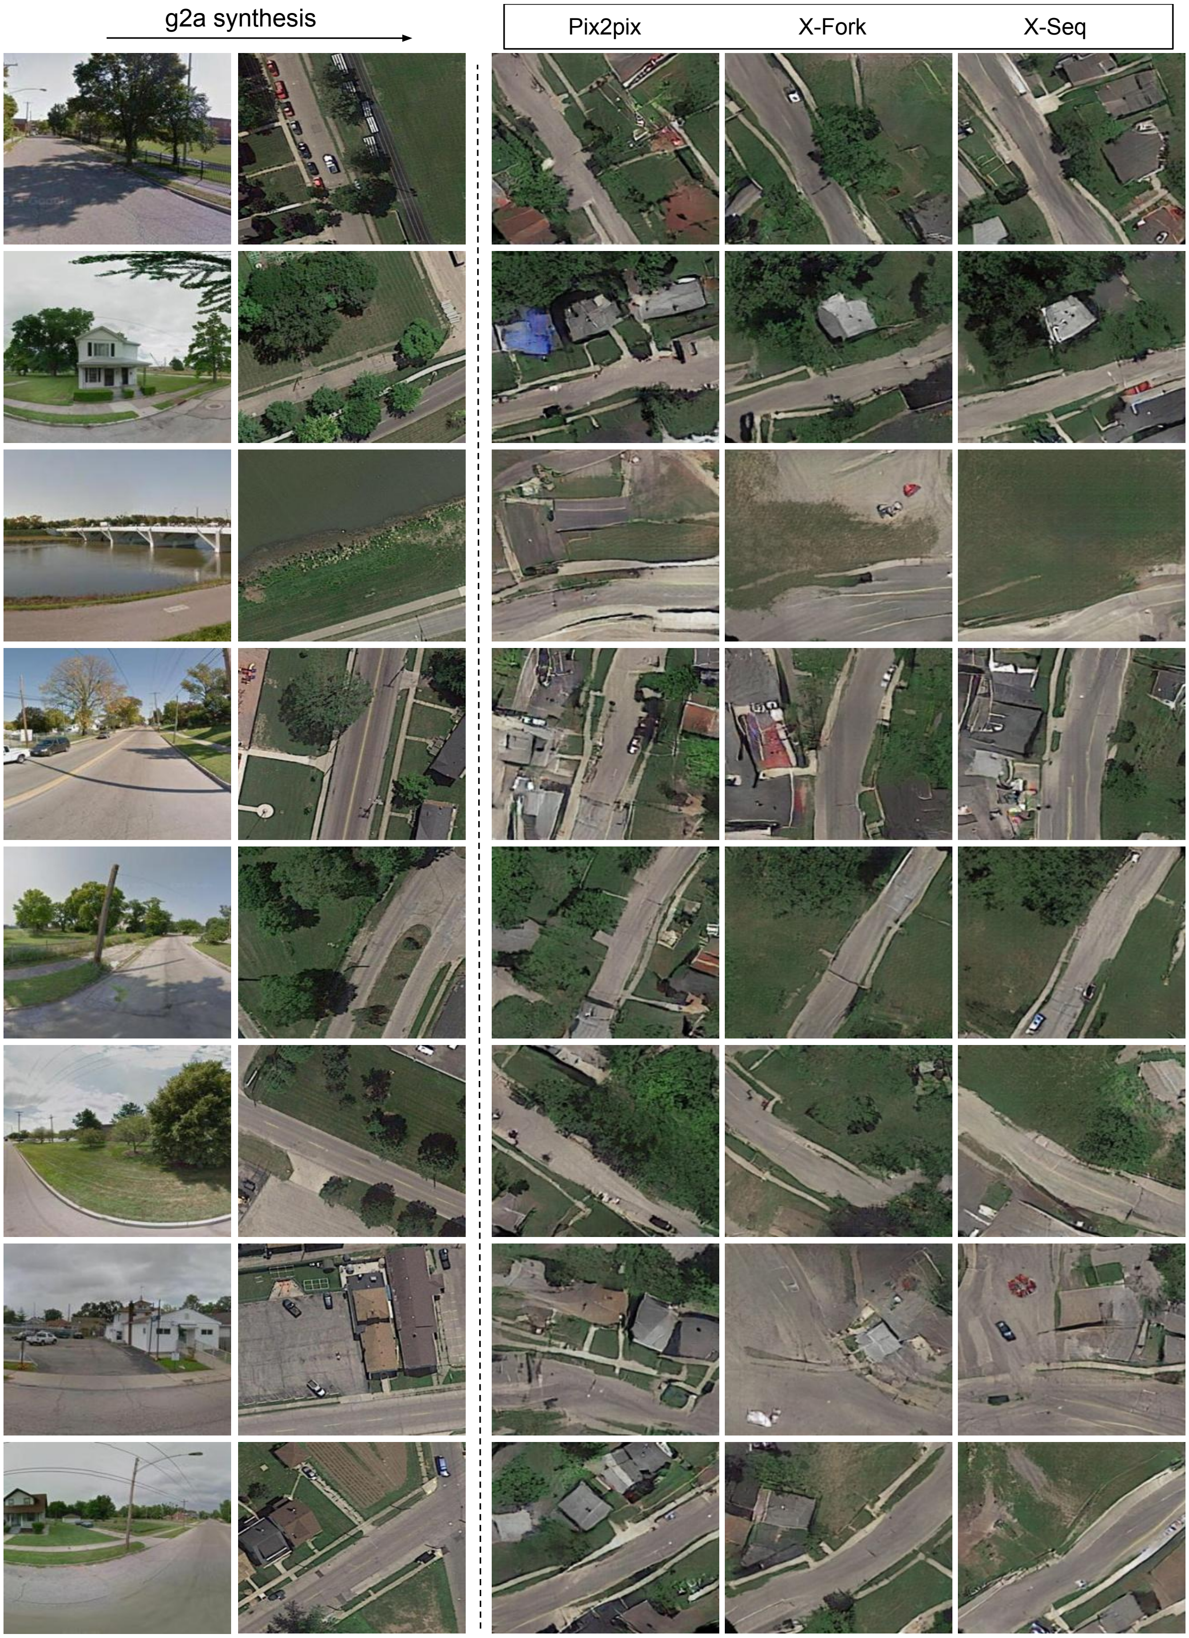


Figure 4: Qualitative results for Ground to Aerial (**g2a**) synthesis using different methods on Dayton dataset.

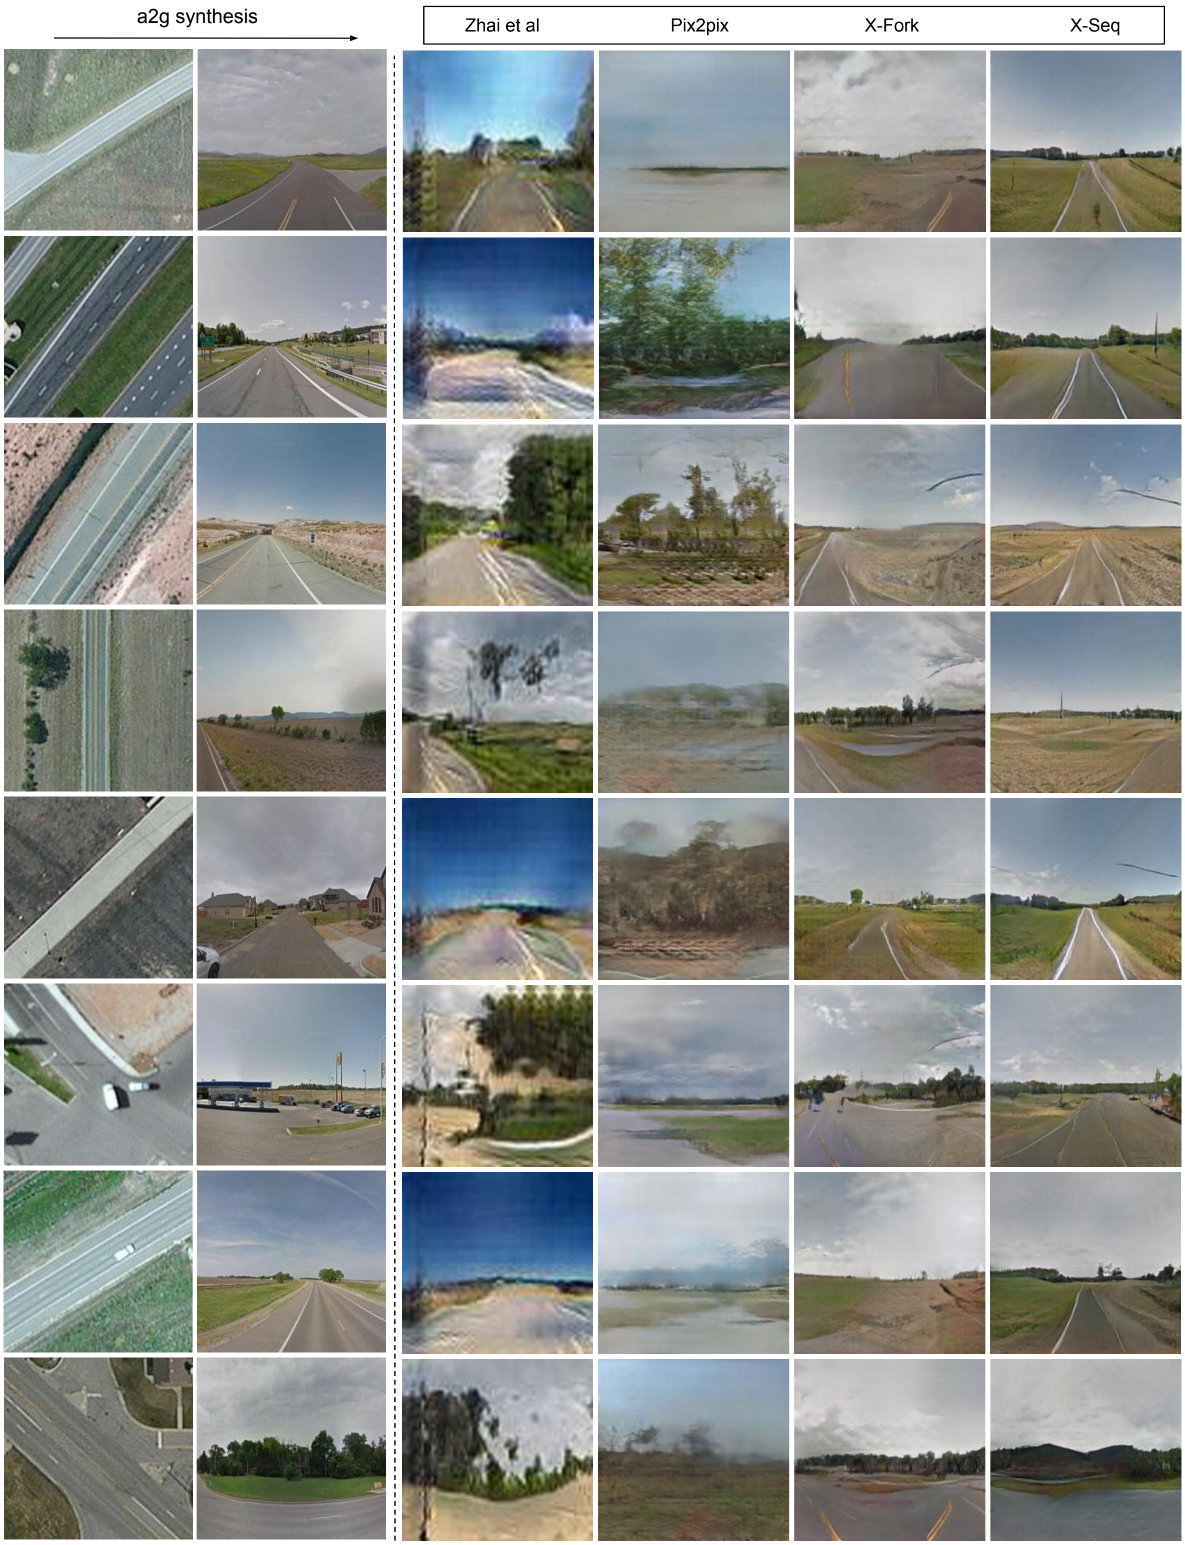


Figure 5: Qualitative results for Aerial to Ground level (a2g) synthesis using different methods on CVUSA dataset.
